# Supplementary material for: Widely tunable, non-degenerate three-wave mixing microwave device operating near the quantum limit
Source: arXiv:1202.1315 ancillary file (2012-02-06)
Supplement: Supplementary file 1 [file Supplementary_material.pdf]

**Supplementary information:**  
**Widely tunable, non-degenerate three-wave mixing microwave  
device operating near the quantum limit**

N. Roch,<sup>1</sup> E. Flurin,<sup>1</sup> F. Nguyen,<sup>1,\*</sup> P. Morfin,<sup>1</sup> P.  
Campagne-Ibarcq,<sup>1</sup> M. H. Devoret,<sup>2,1,3</sup> and B. Huard<sup>1,†</sup>

<sup>1</sup>*Laboratoire Pierre Aigrain, Ecole Normale Supérieure,  
CNRS (UMR 8551), Université P. et M. Curie,*

*Université D. Diderot 24, rue Lhomond, 75231 Paris Cedex 05, France*

<sup>2</sup>*Collège de France, 11 Place Marcelin Berthelot, F-75231 Paris Cedex 05, France*

<sup>3</sup>*Department of Applied Physics, Yale University,  
PO Box 208284, New Haven, CT 06520-8284*

## EFFECT OF STRAY INDUCTANCES ON THE RESONANCE FREQUENCY

The goal of this section is to quantitatively determine the role of stray inductances, on the resonance frequencies of the three-wave mixer.

### Without stray inductance

We can fit the resonance frequency of the signal cavity as a function of the applied flux using the equations from the letter (See Fig.1).

$$\omega_{X,Y} = \omega_{X,Y}^0 \frac{\pi^2 L_{X,Y}^{\lambda/2}/2}{\pi^2 L_{X,Y}^{\lambda/2}/2 + L_{X,Y}(\varphi_{ext})} \quad (1)$$

where  $L_{X,Y}^{\lambda/2} = 2Z_0/(\pi\omega_{X,Y}^0)$  is the lumped-element equivalent inductance,  $L_{X,Y} = \varphi_0^2 (E_L/2 + E_J \cos \varphi_J)^{-1}$  is the ring inductance and  $Z_0$  the characteristic impedance of the bare microstrip resonators.  $E_L$  is defined as  $\varphi_0^2/L$  and the Josephson energy as  $E_J = \varphi_0 I_0 = \varphi_0^2/L_J^0$ . From the geometry, we establish  $Z_0 = 45 \, \Omega$ .

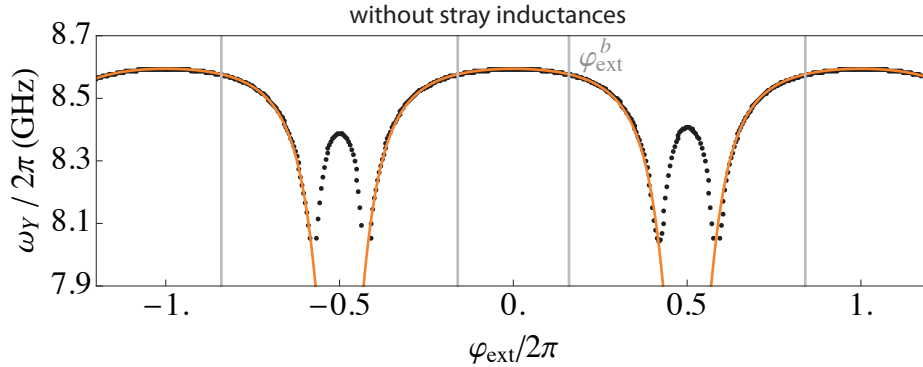

FIG. 1: Dots: Measured resonance frequency  $\omega_Y$  of the signal cavity as a function of flux applied to the ring modulator without pump. Solid orange line: fit of  $\omega_Y$  using Eqs. (1) with  $\omega_Y^0/2\pi = 8.66$  GHz,  $L = 18$  pH and  $L_J^0 = 38$  pH corresponding to  $I_0 = 8.6 \, \mu\text{A}$ . Vertical gray bars indicate the predicted boundaries between small and wide arches using these fit parameters. Neglecting stray inductances, the model does not predict the measured boundaries.

However the actual values of the Josephson and central inductances cannot be deduced accurately from this fitting procedure due to the effect of the non-negligible inductances in

series with the junctions. Moreover, without taking into account these stray inductances, the flux  $\varphi_{\text{ext}}^b$  at the boundary between wide and small arches should be given by

$$L_Z = 0 \Leftrightarrow \cos \varphi_{\text{ext}}^b = -E_L/4E_J \approx 0.53.$$

This value  $\varphi_{\text{ext}}^b/2\pi \equiv \pm 0.16(\text{mod } 1)$  is far from the measured crossover between both arches in Fig.1. This is a clear indication of the need to take into account stray inductances in the model.

### With stray inductances

These stray inductances correspond to the 40  $\mu\text{m}$ -long straight aluminum strips connecting the junctions to the resonators as shown on Fig.2 given by  $L_S = \mu_0 l \approx 50$  pH.

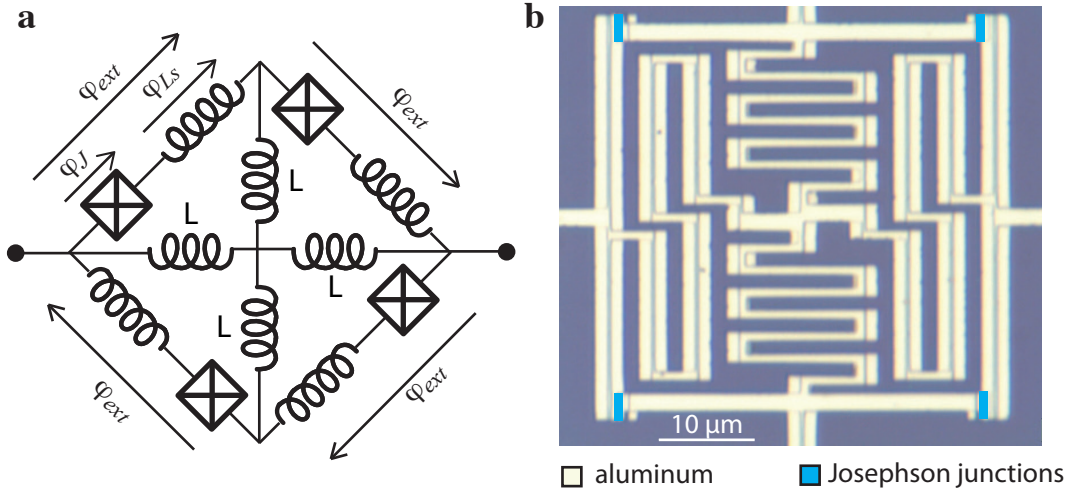

FIG. 2: **a.** Device schematic: four linear inductances  $L$  cross-link a ring of four Josephson junctions in series with stray inductances  $L_S$ . **b.** Optical microscope image of the ring modulator.

We will see below how the model can be modified to take into account these stray inductances. The ring inductances as seen from the X and Y modes can be determined from the electrical circuit.

$$L_{X,Y} = 2(L_J + L_S) // 2(L_J + L_S) // 2L = \frac{1}{\frac{1}{L_J(\varphi_J) + L_S} + \frac{1}{2L}}$$

$$\Leftrightarrow L_{X,Y} = \varphi_0^2 \left( \frac{E_L}{2} + \frac{E_J \cos \varphi_J}{1 + \frac{E_J}{E_{L_S}} \cos \varphi_J} \right)^{-1} \quad (2)$$

where  $E_{L_S} = \varphi_0^2/L_S$  is the stray inductance energy and  $L_J(\varphi_J) = \varphi_0^2/E_J \cos \varphi_J$  is the Josephson inductances.

Similarly, the ring inductances as seen from the Z mode is given by

$$L_Z = \varphi_0^2 \left( \frac{E_L}{4} + \frac{E_J \cos \varphi_J}{1 + \frac{E_J}{E_{L_S}} \cos \varphi_J} \right)^{-1}. \quad (3)$$

The wide arches of figure 1 correspond to the range of flux for which  $L_Z(\varphi_{ext}) > 0$ . In this case, the current through the central inductances is zero and the external arms are phase biased to  $\varphi_{ext}$ , by the magnetic flux as shown in Fig.2:  $\varphi_{ext} = \varphi_{L_S} + \varphi_J$ . Besides current conservation along these external arms gives

$$E_{L_S} \varphi_{L_S} = E_J \sin \varphi_J$$

Consequently, for  $E_J \ll E_{L_S}$  small enough,  $\varphi_J$  can be expanded as

$$\begin{aligned} \varphi_J &= \varphi_{ext} - \frac{E_J}{E_{L_S}} \sin \varphi_J \\ &\approx \varphi_{ext} - \frac{E_J}{E_{L_S}} \sin \varphi_{ext} + \frac{1}{2} \left( \frac{E_J}{E_{L_S}} \right)^2 \sin 2\varphi_{ext} \\ \Leftrightarrow \varphi_J &= \varphi_{ext} - \frac{E_J}{E_{L_S}} \sin \varphi_{ext} + O\left(\left(\frac{E_J}{E_{L_S}}\right)^2\right) \end{aligned} \quad (4)$$

We can now use equations (1,2,4) to describe quantitatively the wide arches of Fig.1. The only fit parameters are the resonance frequency of the bare resonator  $\omega_Y^0/2\pi = 8.82$  GHz, the Josephson critical current  $I_0 = 1.9 \mu\text{A}$  and the central inductance  $L = 49$  pH. Due to the mutual coupling of the meander geometry, the central inductances are reduced compared to a straight geometry. These three fit parameters are consistent with their expected values from geometrical considerations.

Taking into account stray inductances, the flux  $\varphi_{ext}^b$  at the boundary between wide and small arches is predicted to be given by

$$L_Z = 0 \Leftrightarrow \cos(\varphi_J(\varphi_{ext}^b)) = -\frac{E_L/E_J}{4 + E_L/E_{L_S}} = -\frac{L_J^0}{4L + L_S}$$

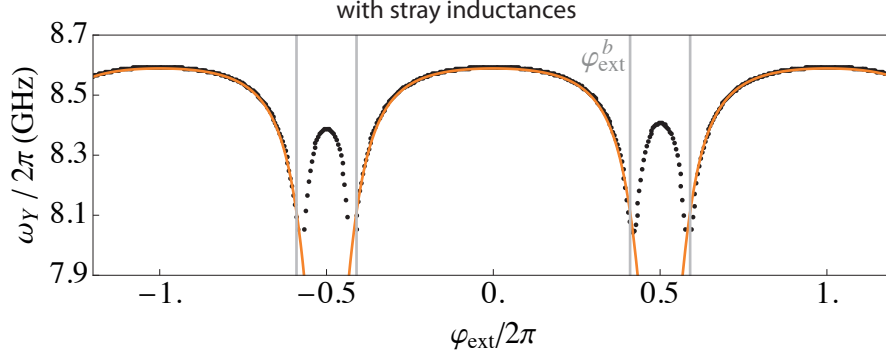

FIG. 3: **a.** Dots: Measured resonance frequency  $\omega_Y$  of the signal cavity as a function of flux applied to the ring modulator without pump. Solid orange line: fit of  $\omega_Y$  taking into account the stray inductances using Eqs. (1), (3) and (5) by fixing  $L_S = 50$  pH and  $Z_0 = 45$   $\Omega$  with  $\omega_Y^0/2\pi = 8.82$  GHz,  $L = 49$  pH and  $L_J^0 = 170$  pH corresponding to  $I_0 = 1.9$   $\mu$ A . Vertical gray bars indicate the predicted boundaries between small and wide arches using these fit parameters.

where  $\varphi_{\text{ext}} = \varphi_J + E_J \sin \varphi_J / E_{L_S}$ . Using the fit parameters above, we get  $\cos(\varphi_J(\varphi_{\text{ext}}^b)) = -0.69$  so that  $\varphi_{\text{ext}}^b/2\pi \equiv \pm 0.41(\text{mod } 1)$ . This is in quantitative agreement with the measured boundary of Fig.3.

---

\* Present address: National Institute of Standards and Technology, 325 Broadway, Boulder CO 80305

† corresponding author: `benjamin.huard@ens.fr`
